# Supplementary material for: Data-Driven Analysis of AI in Medical Device Software in China: Trends of Deep Learning and Traditional AI Based on Regulatory Data
Source: arXiv:2411.07378 source file (2026-04-24)
Supplement: Supplementary file 2 [file Appendix_2.pdf]

| Company name          | Product name                  | Algorithm     | Medical Specialty            | Registration special pathw | Classification | Functional Category                              |
|-----------------------|-------------------------------|---------------|------------------------------|----------------------------|----------------|--------------------------------------------------|
| INNERMED              | VBN-001DV                     | Deep Learning | Otolaryngology               | Normal pathway             | Class II       | Image/Data Processing Software                   |
| Xunfel Healthcare     | Insight                       | General AI    | Respiratory                  | Normal pathway             | Class III      | Decision Support Software - auxiliary detection  |
| Demetics Medical Tech | AI-SONIC-TH-I                 | General AI    | Endocrinology                | Normal pathway             | Class III      | Decision Support Software - auxiliary diagnosis  |
| United-Imaging        | uAI-HematomaCare              | Deep Learning | Neurology                    | Innovation pathway         | Class III      | Decision Support Software - Clinical triage      |
| guiji                 | AIDRscreening                 | Deep Learning | Ophthalmology/ Endocrinology | Innovation pathway         | Class III      | Decision Support Software - auxiliary diagnosis  |
| Infervision           | InferRead CTA Coronary        | Deep Learning | Radiology                    | Normal pathway             | Class III      | Decision Support Software - auxiliary evaluation |
| Infervision           | InferRead CT Lung-Omni        | Deep Learning | Respiratory                  | Normal pathway             | Class III      | Decision Support Software - auxiliary diagnosis  |
| United-Imaging        | uAI-ChestCare                 | Deep Learning | Respiratory                  | Normal pathway             | Class III      | Decision Support Software - auxiliary diagnosis  |
| Infervision           | InferRead CT Fracture         | Deep Learning | Orthopedics                  | Normal pathway             | Class III      | Decision Support Software - Clinical triage      |
| Tencent               | MY-YD-01                      | General AI    | Ophthalmology                | Innovation pathway         | Class III      | Decision Support Software - auxiliary diagnosis  |
| yizhun                | LCI ADS                       | Deep Learning | Respiratory                  | Normal pathway             | Class III      | Decision Support Software - auxiliary diagnosis  |
| Airdoc                | Airdoc-AIFUNDUS               | Deep Learning | Ophthalmology/ Endocrinology | Innovation pathway         | Class III      | Decision Support Software - auxiliary diagnosis  |
| Demetics Medical Tech | AI-SONIC                      | General AI    | Endocrinology                | Normal pathway             | Class III      | Decision Support Software - auxiliary diagnosis  |
| Infervision           | InferVisual Surgery Planning  | Deep Learning | General Surgery              | Innovation pathway         | Class III      | Decision Support Software - Surgical planning    |
| Zhenhealth            | ZZ-EYE-CDS                    | Deep Learning | Ophthalmology/ Endocrinology | Normal pathway             | Class III      | Decision Support Software - auxiliary diagnosis  |
| Huiying Tech          | HY-AIMI-FX                    | Deep Learning | Orthopedics                  | Normal pathway             | Class III      | Decision Support Software - auxiliary diagnosis  |
| United-Imaging        | uAI-PioneerChest              | Deep Learning | Respiratory                  | Innovation pathway         | Class III      | Decision Support Software - auxiliary diagnosis  |
| United-Imaging        | uAI-Discover-NCP              | Deep Learning | Respiratory                  | Normal pathway             | Class III      | Decision Support Software - Clinical triage      |
| Infervision           | IR-CTA-AN                     | Deep Learning | Neurosurgery                 | Normal pathway             | Class III      | Decision Support Software - Clinical triage      |
| Yukun Tech            | LiverMRDoc                    | Deep Learning | Gastroenterology             | Normal pathway             | Class III      | Decision Support Software - Clinical triage      |
| Yukun Tech            | AneurDoc                      | Deep Learning | Neurosurgery                 | Normal pathway             | Class III      | Decision Support Software - Clinical triage      |
| KFBIO                 | KF-TCTAnalysis                | General AI    | Obstetrics and Gynecology    | Normal pathway             | Class II       | Analysis and Mining Products                     |
| Infervision           | InferRead CT Pneumonia        | Deep Learning | Respiratory                  | Normal pathway             | Class III      | Decision Support Software - Clinical triage      |
| Biomind               | HABMSWCOVID19CN               | Deep Learning | Respiratory                  | Normal pathway             | Class III      | Decision Support Software - Clinical triage      |
| SenseTime             | SenseCare-Lung                | Deep Learning | Respiratory                  | Normal pathway             | Class III      | Decision Support Software - auxiliary diagnosis  |
| Infervision           | InferRead CT Lung-LA          | Deep Learning | Respiratory                  | Normal pathway             | Class III      | Decision Support Software - auxiliary diagnosis  |
| Vistel                | EyeWisdom                     | General AI    | Ophthalmology/ Endocrinology | Normal pathway             | Class III      | Decision Support Software - auxiliary diagnosis  |
| Shukun Chuangzhi      | LungdimensionDoc              | Deep Learning | General Surgery              | Normal pathway             | Class III      | Image/Data Processing Software                   |
| United-Imaging        | uAI-BoneCare                  | Deep Learning | Orthopedics                  | Normal pathway             | Class III      | Decision Support Software - auxiliary diagnosis  |
| Infervision           | InferRead CT Stroke           | Deep Learning | Neurology                    | Normal pathway             | Class III      | Decision Support Software - Clinical triage      |
| VoxelCloud            | VoxelCloud Retina             | General AI    | Ophthalmology/ Endocrinology | Normal pathway             | Class III      | Decision Support Software - auxiliary diagnosis  |
| Yukun Tech            | BoneageDoc                    | Deep Learning | Orthopedics                  | Normal pathway             | Class III      | Decision Support Software - auxiliary diagnosis  |
| Pulse Medical         | AngioPlus Core                | Deep Learning | Cardiology                   | Normal pathway             | Class III      | Analysis and Mining Products                     |
| 91360 Med Tech        | CCAA                          | Deep Learning | Obstetrics and Gynecology    | Normal pathway             | Class III      | Analysis and Mining Products                     |
| Infervision           | IR-CTA-ST                     | Deep Learning | Neurology                    | Normal pathway             | Class III      | Decision Support Software - auxiliary diagnosis  |
| Surgiplan             | EC01                          | Deep Learning | Gastroenterology             | Normal pathway             | Class III      | Decision Support Software - auxiliary diagnosis  |
| Infervision           | InferOperate Abdomen Planning | Deep Learning | Hepatology                   | Normal pathway             | Class III      | Decision Support Software - Surgical planning    |
| EDAN                  | Intelligent ECG Platform      | Deep Learning | Cardiology                   | Normal pathway             | Class III      | Image/Data Processing Software                   |

|            |                     |            |                  |                |          |                                                 |
|------------|---------------------|------------|------------------|----------------|----------|-------------------------------------------------|
| hmibiotech | LiveBoost PC        | General AI | Hepatology       | Normal pathway | Class II | Analysis and Mining Products                    |
| Yujin AI   | YCS                 | General AI | Gastroenterology | Normal pathway | Class II | Decision Support Software - auxiliary diagnosis |
| KFBIO      | KF-Gastric-Analysis | General AI | Gastroenterology | Normal pathway | Class II | Analysis and Mining Products                    |
| KFBIO      | KF-TH-DIAG          | General AI | Endocrinology    | Normal pathway | Class II | Image/Data Processing Software                  |
